# Supplementary material for: Simultaneous Learning of Static and Dynamic Charges
Source: arXiv:2601.03656 source file (2026-05-18)
Supplement: Supplementary file 1 [file si.tex]

\documentclass[aps,superscriptaddress,longbibliography,floatfix]{revtex4}
\usepackage{graphicx}
\usepackage[fleqn]{amsmath}
\usepackage{amssymb}
\usepackage[dvipsnames]{xcolor}
\usepackage[normalem]{ulem}
\definecolor{goodgreen}{rgb}{0.1,0.5,0}
\definecolor{goodred}{rgb}{0.7,0,0}
\usepackage{float}
\usepackage{multirow}
\usepackage{sidecap}

\usepackage{xr-hyper}
\externaldocument{staerk25d_Tcc-electrode}

\usepackage{listings} 

\lstset{ 
  backgroundcolor=\color{white},
  basicstyle=\footnotesize
}

\usepackage{array,mathtools,amssymb,booktabs}

\AtBeginDocument{%
  \heavyrulewidth=.08em
  \lightrulewidth=.05em
  \cmidrulewidth=.03em
  \belowrulesep=.65ex
  \belowbottomsep=0pt
  \aboverulesep=.4ex
  \abovetopsep=0pt
  \cmidrulesep=\doublerulesep
  \cmidrulekern=.5em
  \defaultaddspace=.5em
}

%%%%%%%%%%%%%%%%%%%%%%%%%%%%%%%%%%%%%%%%%%%%%%%%%%%%%%%%%%%%%%%%%%%%%%%%%%%%%%%%

%%%%%%%%%%%%%%%%%%%%%%%%%%%%%%%%%%%%%%%%%%%%%%%%%%%%%%%%%%%%%%%%%%%%%%%%%%%%%%%%%

\usepackage[colorlinks,urlcolor=goodgreen,citecolor=blue,linkcolor=goodred]{hyperref}
\usepackage{bm}
\allowdisplaybreaks
\interfootnotelinepenalty=10000

\usepackage{todonotes} 
\usepackage{cleveref} 
\usepackage{siunitx} 
\usepackage{physics} 
\usepackage{csquotes} 

\usepackage{pgfplots} 
% \usetikzlibrary{external}
% \tikzexternalize[prefix=./tikz_externalized/] % activate and define figures/ as cache folder

\usepackage{import}
\usepackage{xifthen}
\usepackage{pdfpages}
\usepackage{transparent}

\newcommand{%
    
    \import{./figures/}{.pdf_tex}
}[1]{%
    
    \import{./figures/}{#1.pdf_tex}
}

\newcommand{%
    
    \import{./figures/}{.pdf_tex}
}[2]{%
    
    \import{./figures/}{#1.pdf_tex}
}

\renewcommand{\epsilon}{\varepsilon}

\DeclareSIUnit{\calorie}{cal}

%-------------------------------------------------------
  % Syntax for version >= 1.2

% Marcel math notation

\begin{document}

\input{si_content}

\bibliography{
  bibliography/Literature.bib,
  bibliography/philip.bib,
  bibliography/egor.bib
}

\end{document}
